# Supplementary material for: REXPACO ASDI: Joint unmixing and deconvolution of the circumstellar environment by angular and spectral differential imaging
Source: arXiv:2109.12644 source file (2024-10-03)
Supplement: Supplementary file 1 [file REXPACO_ASDI_SUPPLEMENTARY.pdf]

# Joint unmixing and deconvolution for angular and spectral differential imaging *supplementary material*

Olivier Flasseur, Loïc Denis, Éric Thiébaud and Maud Langlois

This supplementary material complements Fig.3 of the main manuscript with detailed results about the statistical models of the nuisance component. Figure 1 gives the empirical distribution of the centered and whitened patches (free from object contribution), for different covariance models: diagonal spatial and spectral covariances (i.e., spatial, spectral and temporal weighting) in the first column; full spatial covariance, diagonal spectral covariance, and temporal weighting in second column; full spectral covariance, diagonal spatial covariance, and temporal weighting in third column; and finally the full spatio-spectral separable model introduced in this work (see equation (4) of the main paper) in the last column.

We recall that if random vectors  $\mathbf{v}_n$  are accurately modeled by a Gaussian distribution with mean  $\boldsymbol{\mu}_n$  and covariance  $\mathbf{C}_n$ , then the centered and whitened vectors  $\mathbf{C}_n^{-1/2}(\mathbf{v}_n - \boldsymbol{\mu}_n)$  should follow  $\mathcal{N}(\mathbf{0}, \mathbf{I})$ . Therefore, we compare a standard Gaussian distribution with the empirical marginal distribution of  $\mathbf{C}_n^{-1/2}(\mathbf{v}_n - \boldsymbol{\mu}_n)$  for the four models investigated in this paper.

Since the nuisance component is much stronger close to the star (center of the field-of-view), we also compare the empirical distribution of centered and whitened patches located near the host star with patches extracted farther away. The same type of representation was given in Fig.4 of [1] on this dataset for three additional models considered in our previous work for exoplanet detection in angular and spectral differential imaging: (i) no covariance; (ii) only spatial covariances; (iii) spatial covariances plus temporal and spectral weighting.

The full spatio-spectral separable model introduced in this paper appears to be the most accurate to describe statistically the fluctuations of the nuisance component.

Note that, whatever the model, the empirical distribution of the centered and whitened patches follows more closely a Gaussian law with zero mean and unit variance far from the star than near the star, which is to be expected given that nuisances are much stronger close to the star, and spatial as well as spectral correlations are higher (see Fig.2 of the main paper).

## References

- [1] O. Flasseur, L. Denis, É. Thiébaud, and M. Langlois, “PACO ASDI: an algorithm for exoplanet detection and characterization in direct imaging with integral field spectrographs,” *Astronomy & Astrophysics*, vol. 637, p. A9, 2020.

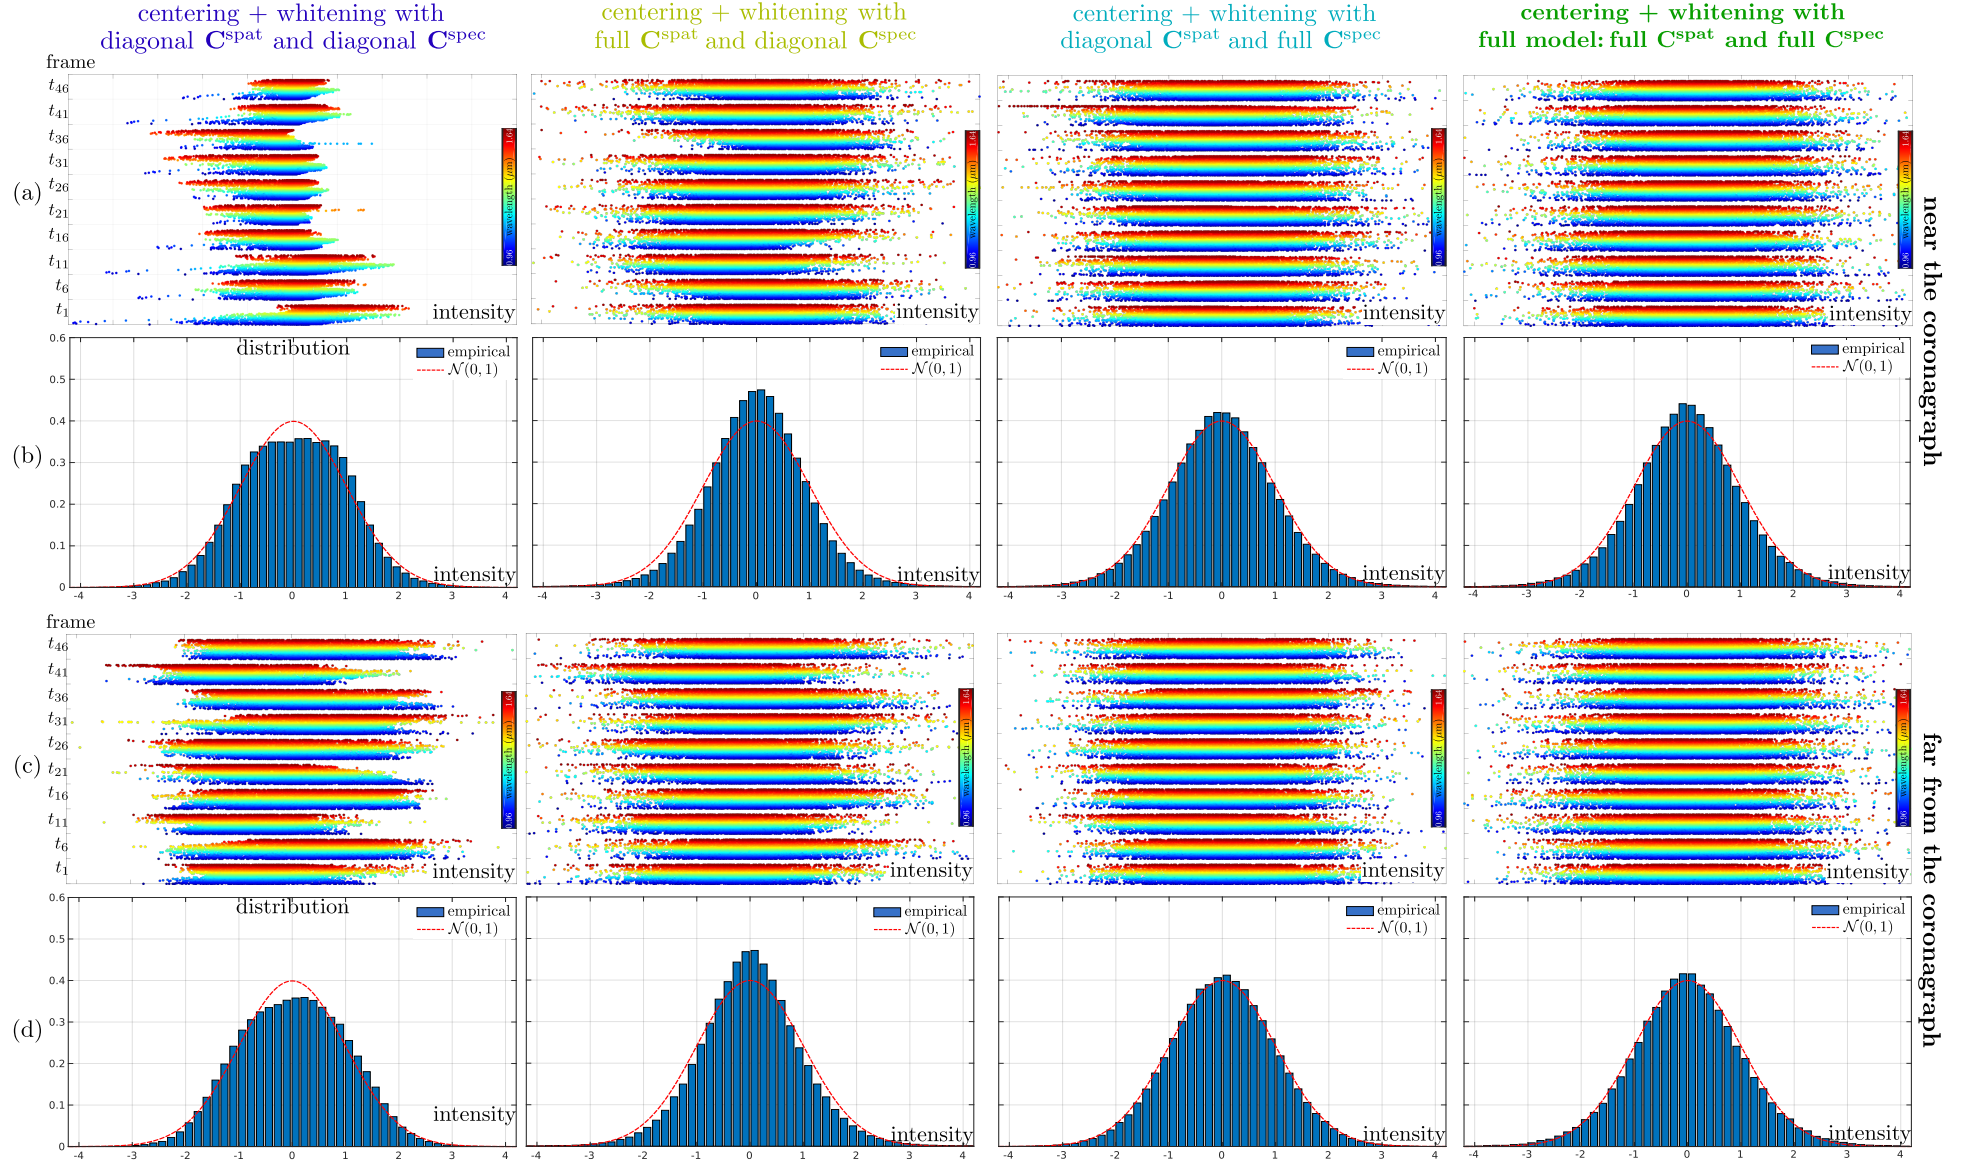

Figure 1: Empirical distribution of the centered and whitened patches: diagonal spatial and spectral covariances in the first column; full spatial covariance, diagonal spectral covariance, and temporal weighting in the second column; full spectral covariance, diagonal spatial covariance, and temporal weighting in the third column; and finally in the last column the full spatio-spectral separable model introduced in this work. Rows a and b: location selected at a small angular separation; rows c and d: location at a larger angular separation. The empirical distribution computed over the whole field of view is given in Fig.3 of the main paper. Patches represented in this figure contain only the contribution from the nuisance component (i.e., no exoplanet or disk).
